# Supplementary material for: Revisiting Pool-based Prompt Learning for Few-shot Class-incremental Learning
Source: arXiv:2507.09183 source file (2025-07-20)
Supplement: Supplementary file 1 [file X_suppl.tex]

\clearpage
\setcounter{page}{1}
\maketitlesupplementary
\setcounter{section}{0} 
\setcounter{figure}{0}  % 重置图片计数器
\setcounter{table}{0}   % 重置表格计数器

\section{Detailed Review of Related Work}

\subsection{Visual Prompting}
Visual Prompt Tuning (VPT)~\cite{jia2022visualprompttuning} pioneered the adaptation of prompt learning to computer vision by introducing learnable prompt tokens into vision transformers. The core principle involves prepending learnable parameters to the input sequence while keeping the backbone frozen, achieving performance comparable to full fine-tuning with only 0.1\% of trainable parameters. This parameter-efficient approach was inspired by prompt learning in Natural Language Processing (NLP)~\cite{brown2020language,liu2021pre}, where it evolved from manual text prompts to learnable continuous vectors~\cite{lester2021power}. The success of prompt learning has also catalyzed various developments in vision-language models, such as CLIP~\cite{radford2021learning} and CoOp~\cite{zhou2022learning}.

\textbf{Efficiency and Adaptability:} DePT~\cite{gao2022visualprompttuningtesttime} optimizes source-initialized prompts for test-time adaptation, while E2VPT~\cite{cheng2023e2vpt} introduces token-wise and segment-wise prompt pruning to reduce parameter overhead. PViT~\cite{zhang2025pvitprioraugmentedvisiontransformer} develops task-specific prompts for multi-task scenarios, and LPT~\cite{dong2023lptlongtailedprompttuning} addresses long-tailed distribution challenges by combining shared and group-specific prompts.

\textbf{Continual Learning Applications:} Learning to Prompt (L2P)~\cite{wang2022learning} made a significant breakthrough by introducing a pool mechanism to maintain shared prompts across tasks. This approach was further enhanced by DualPrompt~\cite{wang2022dualprompt}, which introduced complementary general and expert prompts to capture both task-invariant and task-specific knowledge. These methods have demonstrated superior performance compared to traditional parameter-efficient approaches such as Adapter~\cite{pfeiffer2020adapterfusion} and LoRA~\cite{hu2021lora}. Recent advances include CODA-Prompt~\cite{wang2023codaprompt}, which improves prompt-based continual learning through cross-task knowledge distillation, and S-Prompts~\cite{wang2023spromptslearningpretrainedtransformers}, which explores similar strategies in domain-incremental learning scenarios. The latest HideP~\cite{wang2023hierarchicaldecompositionpromptbasedcontinual} introduces a hierarchical decomposition approach to optimize different components of continual learning separately.

\textbf{Instance-Level Adaptation:} Recent work has focused on addressing the challenge of capturing instance-specific features from different perspectives. InsVP~\cite{liu2024insvp} introduces a dual-level instance visual prompting scheme, which leverages both image-level and feature-level instance-specific information to enhance model recognition capability. Similarly, DAM-VP~\cite{huang2023diversityawaremetavisualprompting} proposes a cluster-level visual prompting method that learns distinct prompt sets for different sample clusters.

Despite these advances, several challenges remain in prompt-based visual learning. Current pool-based prompting methods still struggle with efficient prompt selection and utilization, especially when spatial information plays a vital role in distinguishing fine-grained features. The static nature of prompt pool structures may limit the model's ability to fully leverage task relationships and adapt to novel scenarios. Moreover, the complex interaction between prompts and vision transformer layers requires deeper investigation to optimize knowledge transfer and mitigate catastrophic forgetting. While recent advances have addressed some of these limitations through instance-level adaptation and spatial information utilization, there remains significant room for improvement in prompt pool design and management, particularly in effectively combining local and global spatial information while maintaining model efficiency.

\begin{table*}[t]
    \centering
    \small
    \setlength{\tabcolsep}{2.5pt}
    \begin{tabular}{l|l|r|c|c|c|c|c|c|c}
        \hline
        Dataset & Domain & Images & Classes & Base & Base Setup & Novel & Novel Setup & Train/Test & Source \\
        \hline
        CUB-200 & Fine-grained Birds & 11,788 & 200 & 100 & 100w-30s (3K) & 100 (10/ses) & 10×(10w-5s) & 30/50 & Caltech \\
        iNF200 & Fungi Species & 10,000 & 200 & 100 & 100w-50s (5K) & 100 (10/ses) & 10×(10w-5s) & 50/50 & iNat \\
        FGVCAircraft & Aircraft Variants & 10,000 & 100 & 50 & 50w-30s (1.5K) & 50 (5/ses) & 10×(5w-5s) & 30/50 & FGVC \\
        \hline
    \end{tabular}
    \caption{Detailed dataset configurations for fine-grained visual recognition. Base indicates the number of categories used in initial training (training samples in parentheses), while Novel shows how remaining categories are distributed across 10 incremental sessions. For base training, Train/Test denotes samples per class for training/testing respectively. In novel sessions, we consistently use 5 samples for training and the remaining for testing. The setup format (N-way-K-shot) specifies N categories with K samples per category for both base and novel phases.}
    \label{tab:dataset_details}
\end{table*}

\subsection{FSCIL}

FSCIL represents a sophisticated integration of Few-Shot Learning (FSL) and Class-Incremental Learning (CIL)~\cite{akyürek2022subspaceregularizersfewshotclass}. This paradigm inherits the fundamental challenge of FSL in learning from limited samples, while simultaneously addressing the CIL requirement of maintaining model performance on previously learned tasks as new classes are incrementally introduced.
 
\textbf{Structure-based and Dynamic Network Methods.}
Few-Shot Class-Incremental Learning (FSCIL) was pioneered by Tao et al.~\cite{tao2020fscil}, who introduced a neural gas network to preserve topological relationships between classes. This seminal work laid the foundation for subsequent research, notably CEC~\cite{Zhang_2021_CVPR}, which advanced the field by introducing a class-specific classifier architecture integrated with a graph-based model for efficient inter-classifier information propagation and adaptation. Recent developments in this domain have witnessed a significant shift towards dynamic network architectures, encompassing several key directions: dynamic backbone structures (DSN)~\cite{dynamicBackbone}, structure fusion mechanisms (FeSSSS)~\cite{Ahmad_2022_CVPR}, adaptive sub-networks (SoftNet)~\cite{kang2023softsubnetworkfewshotclassincremental}, and ensemble-based frameworks (LEC-Net)~\cite{yang2021learnableexpansionandcompressionnetworkfewshot}. State-of-the-art methods such as EM~\cite{zhu2024enhancedfewshotclassincrementallearning} have demonstrated the remarkable efficacy of dynamic architectural adaptation in addressing the fundamental challenges of FSCIL.

\textbf{Knowledge Distillation and Replay-Based Methods.}
A significant body of research in FSCIL focuses on knowledge preservation through replay buffers or feature generation mechanisms. LCwoF~\cite{kukleva2021lcwof} and SKD~\cite{rajasegaran2020self} pioneered this direction by incorporating feature pyramid architectures to enhance knowledge preservation capabilities. Building upon this foundation,~\cite{Shankarampeta2021FewShotCI} employed Generative Adversarial Networks to synthesize features, effectively addressing the data scarcity challenge inherent in few-shot scenarios. Recent advances have further refined these approaches: CABD~\cite{10203568CABD} introduced class-aware bilateral distillation, facilitating knowledge transfer between base and novel classes through a sophisticated distillation framework, while UaD-CE~\cite{cui2023uncertainty} enhanced performance through an innovative combination of reference model distillation and uncertainty-aware adaptive mechanisms. While these methods demonstrate promising results, they typically necessitate additional computational resources for storing historical samples or maintaining teacher models.

\textbf{Feature Space-based Methods.}
Early explorations in feature space optimization for FSCIL include LIMIT~\cite{zhou2023few} and WaRP~\cite{kim2023warping}. iCaRL~\cite{rebuffi2017icarlincrementalclassifierrepresentation} introduced a practical strategy for simultaneously learning classifiers and feature representations in the class-incremental setting. FOSTER~\cite{wang2022fosterfeatureboostingcompression} advanced this direction through a two-step paradigm of feature boosting and compression, effectively addressing the performance decline in new classes. Building upon these foundations, FACT~\cite{zhou2022forward} introduced Forward Compatible Training, an innovative approach that reserves representation space through strategic prototype placement. TEEN~\cite{wang2023fewshotclassincrementallearningtrainingfree} proposed a training-free prototype calibration strategy to address the misclassification of new classes into similar base classes. RDI~\cite{zhou2024delvebasenovelconfusionredundancy} further investigated the base-novel confusion problem by decoupling label-irrelevant redundancies in both feature and pixel spaces. ALICE~\cite{peng2022fewshotclassincrementallearningopenset} advanced this direction by emphasizing both feature space compactness and diversity, while SAVC~\cite{song2023learning} incorporated semantic knowledge through virtual class generation.

\textbf{Meta Learning-based and Optimization-based Methods.}
Meta learning and optimization techniques have emerged as powerful approaches in FSCIL, incorporating various regularization strategies and adaptive loss functions. SPPR~\cite{zhu2021selfpromotedprototyperefinementfewshot} enhances feature representation through an innovative prototype refinement strategy, while CLOM~\cite{zou2022marginbasedfewshotclassincrementallearning} introduces a novel cosine loss with negative margin to promote shareable feature learning. C-FSCIL~\cite{hersche2022cfscil} proposes quasi-orthogonal prototype alignment, and Comp-FSCIL~\cite{zou2024compositionalfewshotclassincrementallearning} introduces a cognitive-inspired approach utilizing primitive composition and reuse modules based on set similarities. NC-FSCIL~\cite{yang2023neural} employs dot-regression loss to optimize feature-prototype alignment. Earlier contributions include MetaFSCIL~\cite{9878925MetaFSCIL} and FSLL~\cite{mazumder2021fewshotlifelonglearning}, which established fundamental meta-learning frameworks for incremental few-shot scenarios.

\textbf{Pretrained Model-based Methods.}
Recent advances in FSCIL have increasingly leveraged the remarkable capabilities of pre-trained models. Several pioneering works~\cite{D_Alessandro_2023,huang2024learningpromptdistributionbasedfeature,yoon2023imageobjectspecificpromptlearningfewshot} have explored multi-modal approaches by incorporating CLIP~\cite{radford2021learningtransferablevisualmodels}, establishing novel paradigms for feature alignment between visual and textual modalities. In parallel, significant progress has been made in utilizing Vision Transformers for FSCIL tasks. ASP~\cite{liu2024fewshotclassincrementallearning} demonstrates the effectiveness of this approach by employing a fixed pre-trained backbone while encoding task-invariant knowledge in learnable prompts, effectively addressing the stability-plasticity dilemma. Yourself~\cite{tang2024rethinking} further advances this direction through an innovative feature rectification module, while Approximation~\cite{Wang2024OnTA} establishes comprehensive guidelines for mitigating transfer and consistency risks. A significant breakthrough came with PriViLege~\cite{park2024pretrainedvisionlanguagetransformers}, which effectively addresses catastrophic forgetting through its novel PKT module and semantic knowledge distillation mechanism. Our work builds upon these recent advances, further exploring the potential of pre-trained models in incremental learning scenarios.

\section{Empirical Setup}
\subsection{Experimental Datasets}
We first discuss our dataset selection rationale, focusing on distribution overlap concerns with pre-trained weights. Then we present our three benchmark datasets and their partitioning protocols, followed by evaluation metrics.

\subsubsection{Dataset Selection Rationale}
CIFAR-100~\cite{Krizhevsky2009LearningML}, CUB-200~\cite{Wah2011TheCB}, and miniImageNet~\cite{vinyals2017matchingnetworksshotlearning} have served as standard benchmark datasets in the field. However, we identify a critical limitation in their evaluation capacity for our context. Given that our approach leverages ImageNet pre-trained weights—a common practice shared by~\cite{park2024pretrainedvisionlanguagetransformers},~\cite{Wang2024OnTA},~\cite{tang2024rethinking},~\cite{liu2024fewshotclassincrementallearning}, and~\cite{FineFMPL}—we find that CIFAR-100 and CUB-200 share substantial distribution similarities with ImageNet. This overlap raises concerns about potential data leakage, particularly when applying pre-trained weights to miniImageNet (a subset of ImageNet), which could lead to artificially enhanced performance metrics.

To ensure a more rigorous evaluation of our proposed method, we extend our experiments to two challenging fine-grained datasets: FGVCAircraft~\cite{maji2013finegrainedvisualclassificationaircraft} and a carefully selected subset from iNaturalist (Fungi) ~\cite{VanHorn2018iNaturalist}. Specifically, we work with the first 200 fungal species classes from iNaturalist, referred to as iNF200. These datasets offer distinct visual distributions from ImageNet, enabling a more comprehensive assessment of our method's generalization abilities.

\begin{figure}[t]
    \centering
    \begin{tabular}{@{}c@{\hspace{1mm}}c@{\hspace{1mm}}c@{}}
        \includegraphics[width=0.12\textwidth]{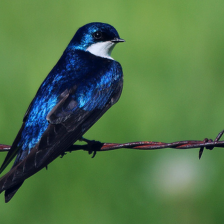} &
        \includegraphics[width=0.12\textwidth]{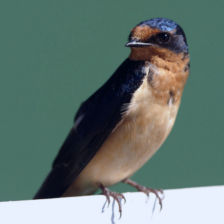} &
        \includegraphics[width=0.12\textwidth]{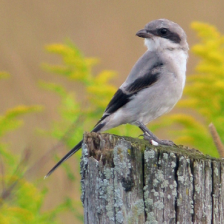} \\
        \includegraphics[width=0.12\textwidth]{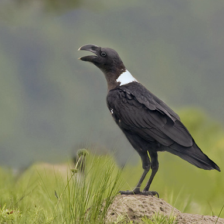} &
        \includegraphics[width=0.12\textwidth]{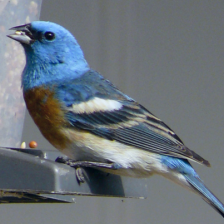} &
        \includegraphics[width=0.12\textwidth]{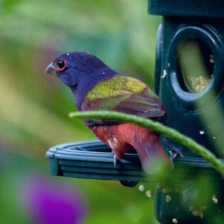} \\
        \includegraphics[width=0.12\textwidth]{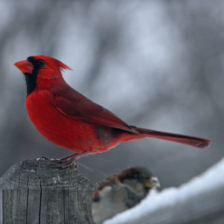} &
        \includegraphics[width=0.12\textwidth]{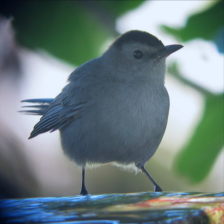} &
        \includegraphics[width=0.12\textwidth]{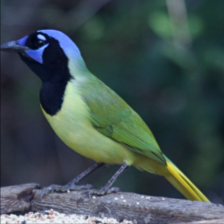}
    \end{tabular}
    \caption{Samples of CUB-200.}
    \label{fig:cub_samples}
\end{figure}

\subsubsection{Benchmark Datasets.}
\textbf{CUB-200} (Caltech-UCSD Birds) is a fine-grained visual classification dataset comprising 200 bird species with a total of 11,788 images, with sample images shown in Figure~\ref{fig:cub_samples}. In our incremental learning setup, we designate the first 100 species as base classes. The remaining classes are evenly distributed across 10 incremental sessions, with each session introducing 10 novel species. Following the few-shot learning paradigm, we utilize 5 samples per class during training, establishing a 10-way 5-shot incremental learning scenario.

\textbf{FGVCAircraft} presents a challenging collection of 10,000 aircraft images spanning 100 distinct aircraft variants, with representative samples shown in Figure~\ref{fig:aircraft_samples}. We structure our experiments by allocating 50 variants as base classes, with the remaining 50 variants distributed across 10 incremental learning sessions. Each session incorporates 5 new aircraft variants, and similar to our other experiments, we maintain a 5-shot learning protocol, resulting in a 5-way 5-shot incremental learning framework.

\begin{figure}[t]
    \centering
    \begin{tabular}{@{}c@{\hspace{1mm}}c@{\hspace{1mm}}c@{}}
        \includegraphics[width=0.12\textwidth,height=0.12\textwidth]{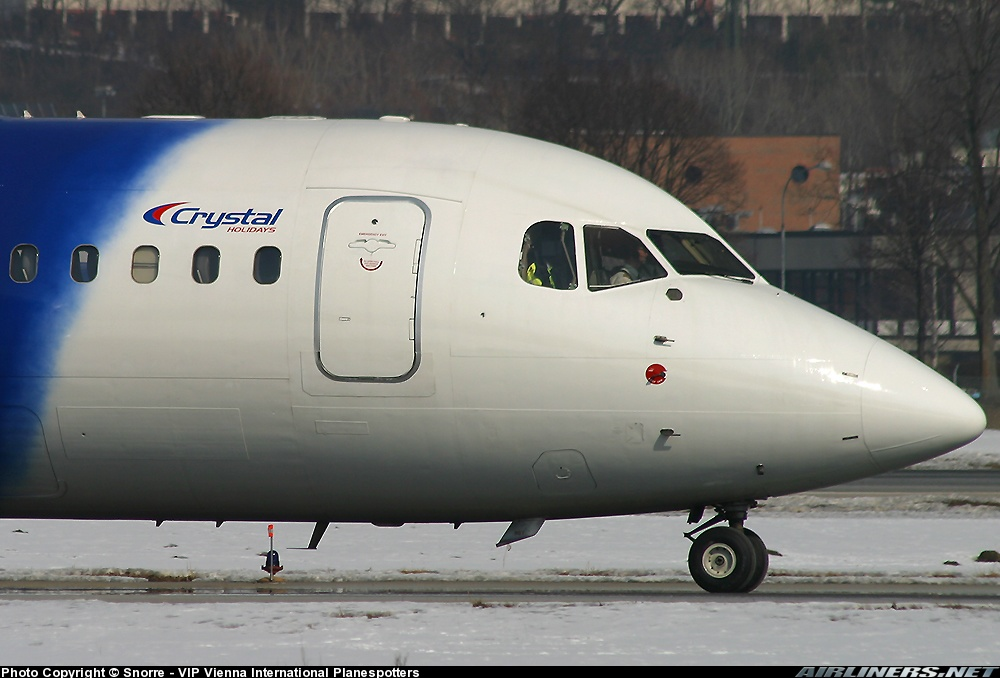} &
        \includegraphics[width=0.12\textwidth,height=0.12\textwidth]{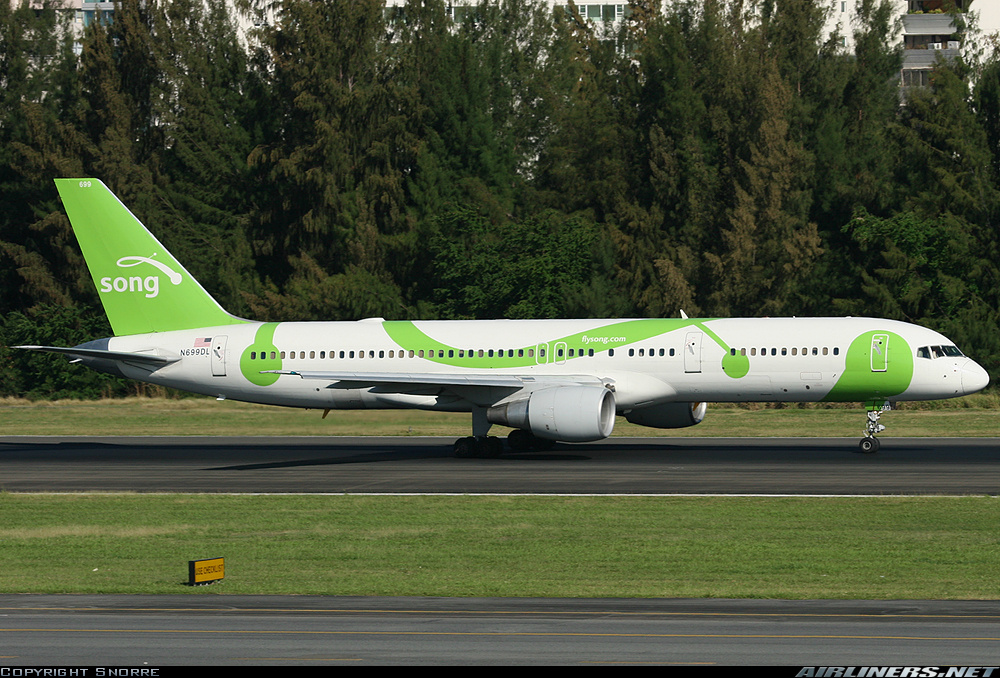} &
        \includegraphics[width=0.12\textwidth,height=0.12\textwidth]{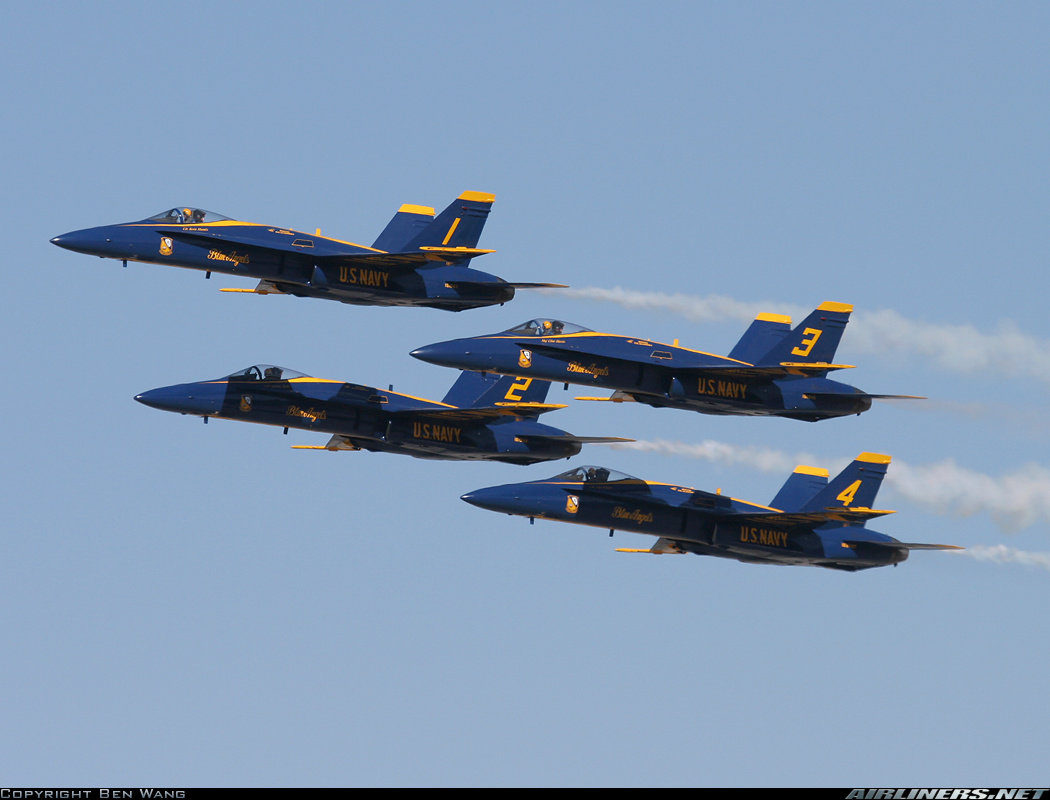} \\
        \includegraphics[width=0.12\textwidth,height=0.12\textwidth]{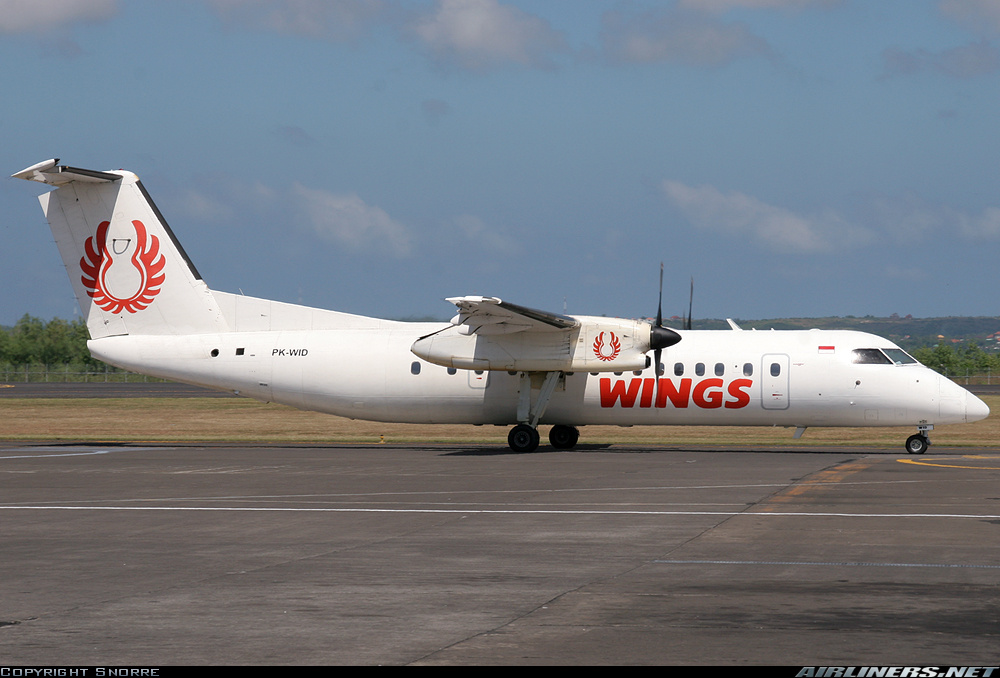} &
        \includegraphics[width=0.12\textwidth,height=0.12\textwidth]{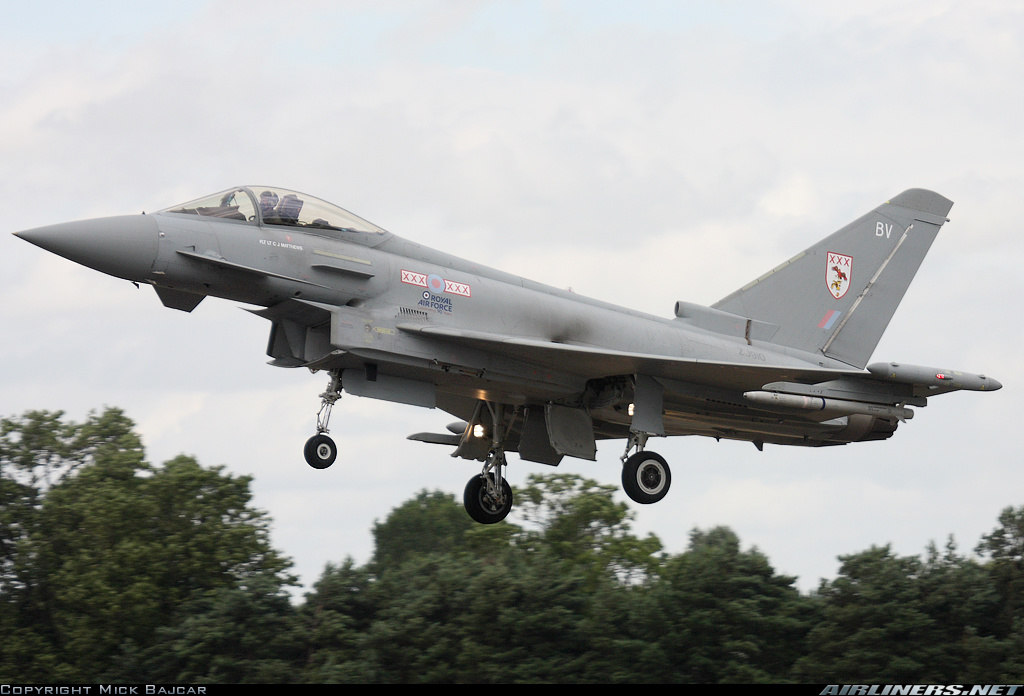} &
        \includegraphics[width=0.12\textwidth,height=0.12\textwidth]{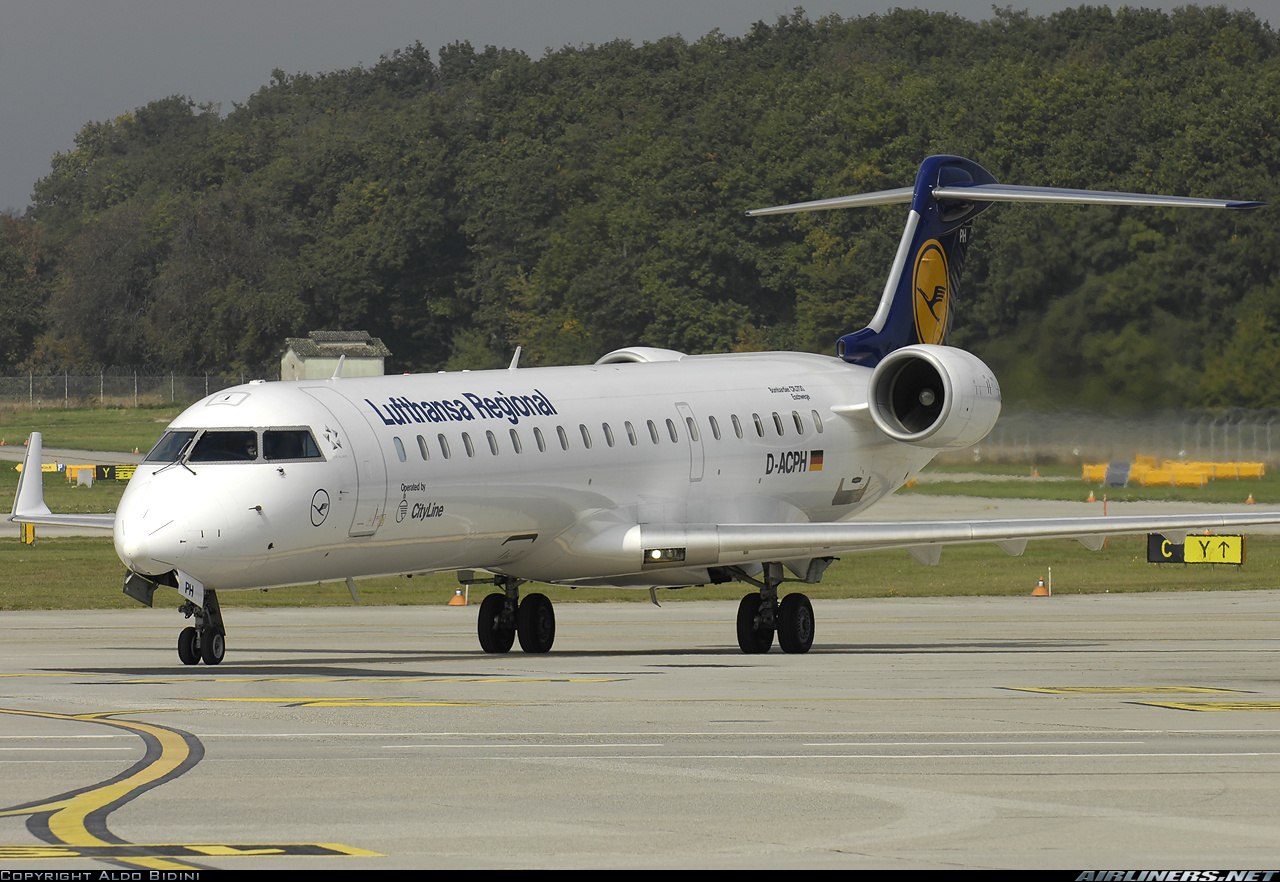} \\
        \includegraphics[width=0.12\textwidth,height=0.12\textwidth]{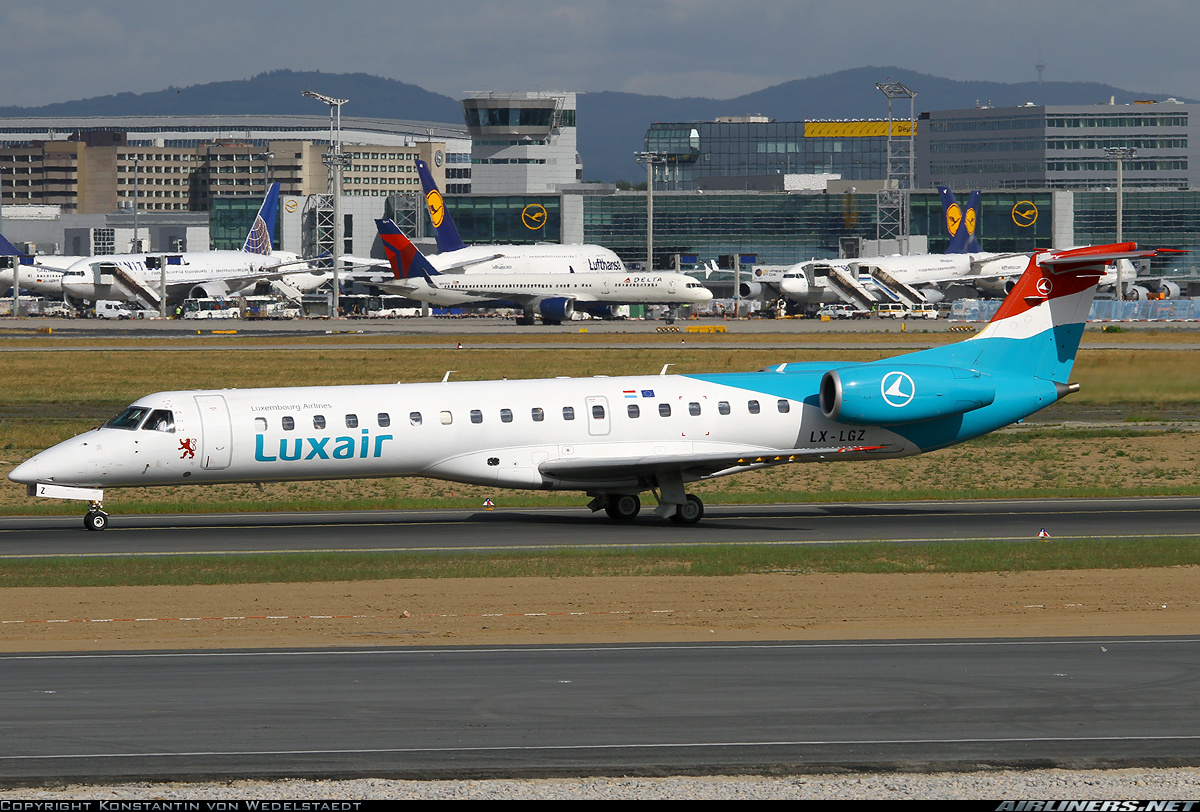} &
        \includegraphics[width=0.12\textwidth,height=0.12\textwidth]{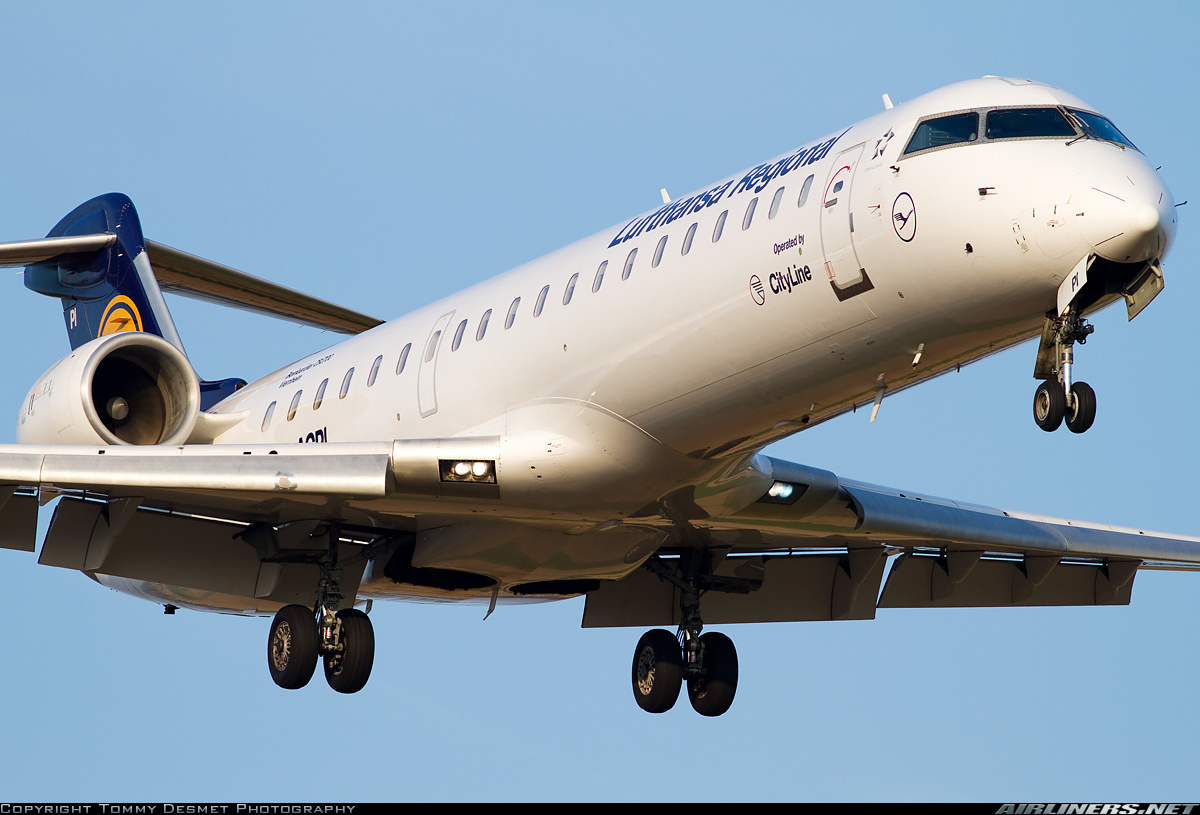} &
        \includegraphics[width=0.12\textwidth,height=0.12\textwidth]{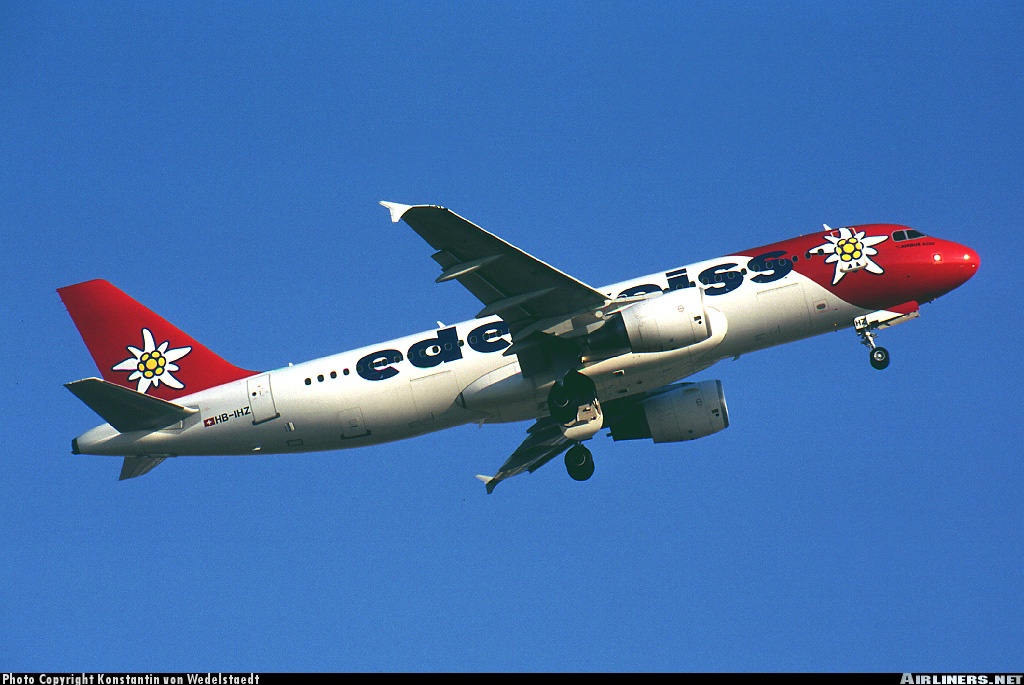}
    \end{tabular}
    \caption{Samples of FGVCAircraft.}
    \label{fig:aircraft_samples}
\end{figure}

\textbf{iNF200} (iNaturalist Fungi-200) represents a carefully curated subset of the iNaturalist dataset's fungi category, with diverse examples illustrated in Figure~\ref{fig:inf_samples}. From the extensive collection of fungal species available in iNaturalist, we select the first 200 classes, each containing 50 images, yielding a total of 10,000 samples. Our experimental protocol assigns the initial 100 species to the base training set. The subsequent 100 species are systematically distributed across 10 incremental sessions, with each session introducing 10 new species. Maintaining consistency with our experimental design, we employ 5 examples per class, establishing a 10-way 5-shot incremental learning configuration.

\begin{figure}[t]
    \centering
    \begin{tabular}{@{}c@{\hspace{1mm}}c@{\hspace{1mm}}c@{}}
        \includegraphics[width=0.12\textwidth,height=0.12\textwidth]{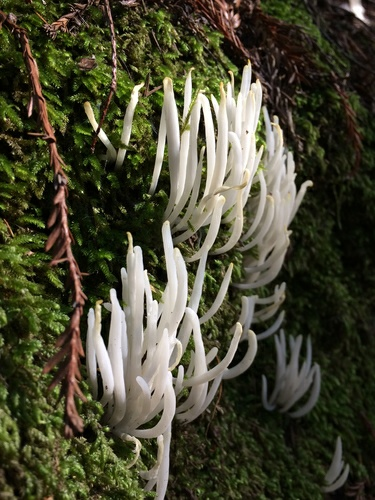} &
        \includegraphics[width=0.12\textwidth,height=0.12\textwidth]{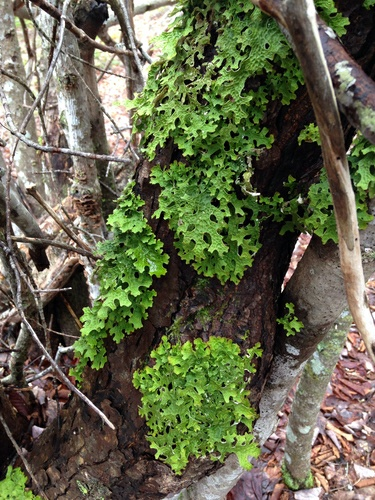} &
        \includegraphics[width=0.12\textwidth,height=0.12\textwidth]{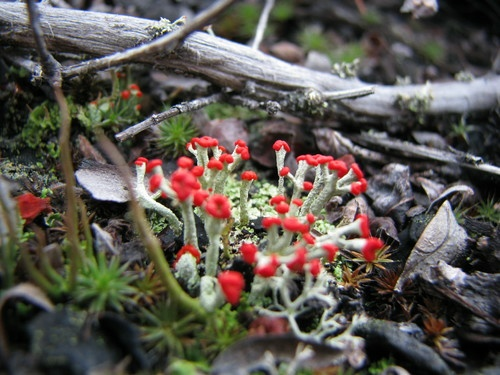} \\
        \includegraphics[width=0.12\textwidth,height=0.12\textwidth]{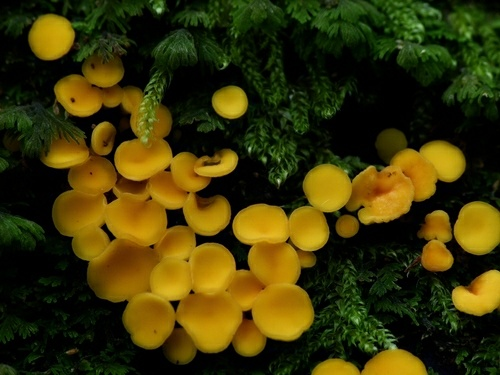} &
        \includegraphics[width=0.12\textwidth,height=0.12\textwidth]{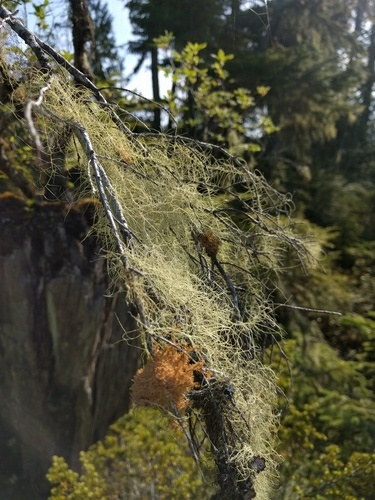} &
        \includegraphics[width=0.12\textwidth,height=0.12\textwidth]{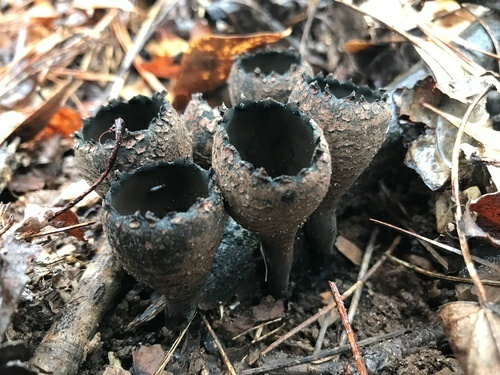} \\
        \includegraphics[width=0.12\textwidth,height=0.12\textwidth]{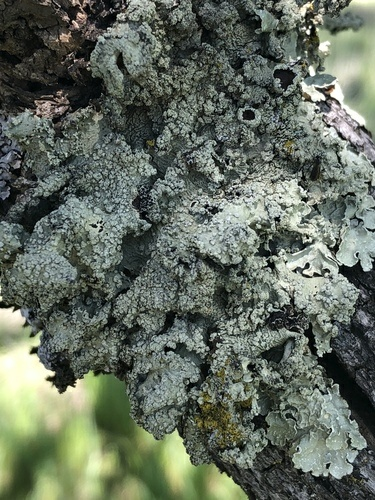} &
        \includegraphics[width=0.12\textwidth,height=0.12\textwidth]{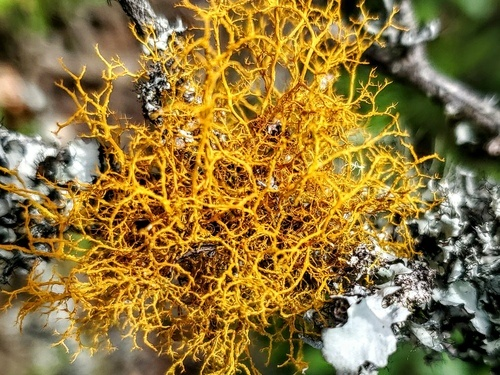} &
        \includegraphics[width=0.12\textwidth,height=0.12\textwidth]{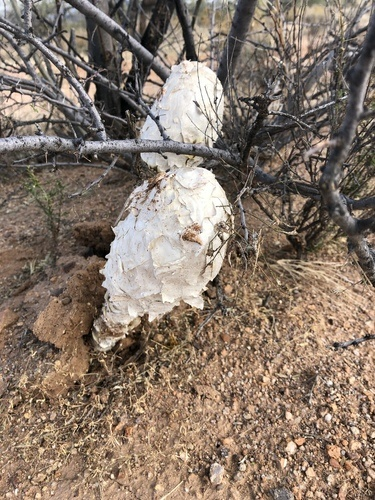}
    \end{tabular}
    \caption{Samples of iNF200.}
    \label{fig:inf_samples}
\end{figure}

\subsubsection{Dataset Partitioning Protocol}
In our experimental design, we adhere to established dataset partitioning protocols to maintain consistency and reproducibility. The CUB-200 dataset follows the division scheme outlined in CEC~\cite{Zhang_2021_CVPR}, while FGVCAircraft and iNF200 are organized according to the protocol described in~\cite{doan2024streamlinedapproachmultimodalfewshot}. This careful consideration in dataset selection and organization provides a robust evaluation framework that effectively addresses the limitations of ImageNet-aligned datasets.

%-------------------------------------------------------------------------
\subsubsection{Evaluation Protocol}
We employ three complementary metrics to comprehensively evaluate our model's performance. For each incremental session $t$, we compute the classification accuracy $A_t$. The overall model performance is assessed through the average accuracy across all sessions, computed as $\text{Avg} = \frac{1}{T}\sum_{i=1}^T A_i$. 

%-------------------------------------------------------------------------
\subsection{Model Implementation}

\subsubsection{Model Architecture and Training Strategy}
Our framework builds upon the Vision Transformer (ViT) architecture, leveraging a model pre-trained on ImageNet-21K as our backbone network. We adopt and extend the Visual Prompt Tuning (VPT) paradigm~\cite{jia2022visualprompttuning}, specifically following the VPT-deep configuration, which has demonstrated superior performance in visual transfer learning tasks. In this setup, we strategically insert learnable prompt tokens between consecutive transformer blocks, enabling fine-grained feature adaptation while maintaining the pre-trained model's robust representational capacity. The prompt parameters are initialized from a normal distribution, following standard practices in transformer-based architectures. 

Following the established practice in few-shot class-incremental learning~\cite{park2024pretrainedvisionlanguagetransformers, Wang2024OnTA, tang2024rethinking, liu2024fewshotclassincrementallearning, FineFMPL}, we keep the pre-trained ViT backbone frozen during the entire learning process. This conventional strategy has proven effective in preventing catastrophic forgetting and maintaining stable feature representations. During training, we only optimize the inserted visual prompts and the prototype-based classifier~\cite{snell2017prototypicalnetworksfewshotlearning}, which aligns with the field's standard approach of selective parameter updating when adapting to novel classes.

\subsubsection{Implementation Details}
The training process consists of two main phases. In the base session, we train the model for 16 epochs with a learning rate of 0.02. This is followed by the novel session, where we fine-tune for 5 epochs with a reduced learning rate of 0.002. For the Local Spatial Pool, we maintain 30 learnable spatial prompts (CNN \& Local Spatial Prompts), each initialized with Kaiming initialization and employing dropout (rate = 0.1) for robust feature extraction. These prompts are trained with a learning rate of 0.001 during the base session.

In the Global Spatial Pool, we design frequency-based prompts organized in concentric regions. These prompts, represented as trainable frequency masks, are optimized throughout both sessions with learning rates of 0.1 and 0.005 for base and novel sessions, respectively. The mask weights are initialized using a normal distribution to ensure balanced initial frequency responses. For adaptive feature integration between local and global spatial information, we introduce two learnable parameters $\alpha_l$ and $\alpha_g$, constrained by $\alpha_l$ + $\alpha_g$ = 1, with both initially set to 0.5. 

These fusion parameters are exclusively optimized during the base session with a learning rate of 0.005, allowing the model to learn optimal combinations of local and global spatial features. To ensure stable convergence, we adopt a CosineAnnealingLR schedule for all learning rate adjustments. All experiments are conducted on a single GPU setup.

\begin{figure}[t]
    \centering
    \includegraphics[width=0.9\columnwidth]{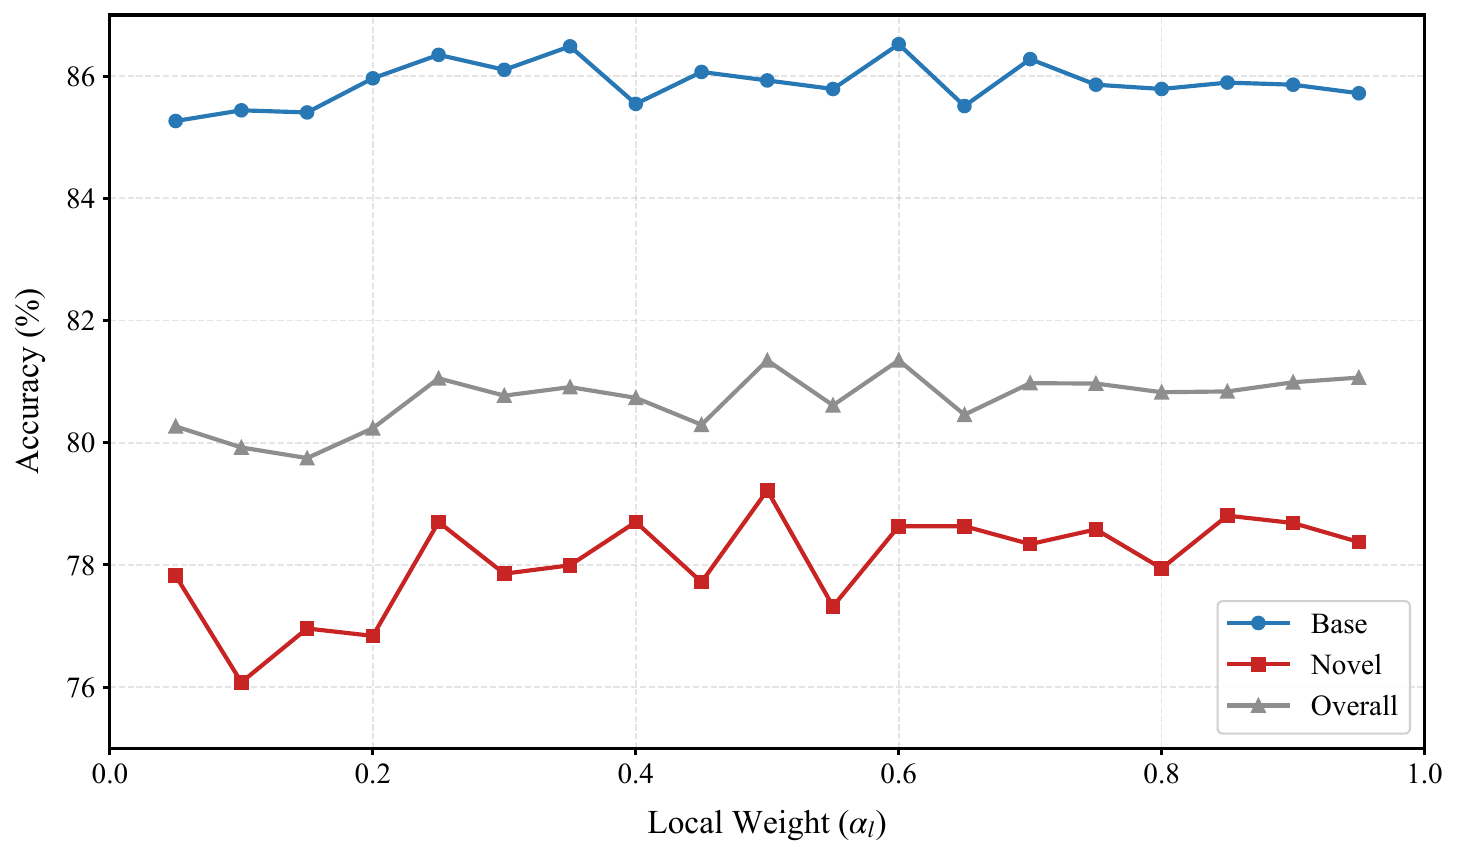}
    \caption{Impact of adaptive weighting mechanism: Analysis of accuracy variations with different initial weight combinations between Local ($\alpha_l$) and Global ($\alpha_g$) Spatial Prompting branches. The model demonstrates robust performance across various weight settings, with optimal performance achieved near balanced weights.}
    \label{fig:weight_analysis}
\end{figure}

%-------------------------------------------------------------------------
%-------------------------------------------------------------------------
\section{Hyperparameter Experiments}

\subsection{Feature Integration Mechanism Study}
\label{subsec:feature_integration}

\subsubsection{Comparison of Integration Strategies}
\begin{table}[t]
\centering
\setlength{\tabcolsep}{4pt}  % 进一步减小列间距
\begin{tabular}{l|c|c}  % 使用l而不是p{width}
\toprule
Integration Strategy & Acc (\%) & $\Delta$ \\
\midrule
Ours (Learnable $\alpha_l$ and $\alpha_g$) & \textbf{81.392} & - \\
\midrule
\multicolumn{3}{l}{\textit{Architecture Variants}} \\
GSP after LSP & 81.242 & -0.150 \\
GSP before LSP & 81.175 & -0.217 \\
Linear layer fusion & 81.260 & -0.132 \\
\midrule
\multicolumn{3}{l}{\textit{Weight Constraints}} \\
Fixed sum constraint ($\alpha_l + \alpha_g = 1$) & 80.179 & -1.213 \\
Only LSP weight learnable & 80.159 & -1.233 \\
Only GSP weight learnable & 80.139 & -1.253 \\
\midrule
\multicolumn{3}{l}{\textit{Advanced Fusion Mechanisms}} \\
Neural network weights & 80.152 & -1.240 \\
Gating mechanism (Sigmoid) & 80.503 & -0.889 \\
Non-linear fusion (MLP) & 80.682 & -0.710 \\
\bottomrule
\end{tabular}
\caption{Ablation study on different feature integration strategies. Our proposed learnable weights achieve the best performance (81.392\%) compared to various alternative fusion mechanisms.}
\label{tab:fusion_ablation}
\end{table}

We evaluate various feature integration strategies to validate our design choice of using learnable weights $\alpha_l$ and $\alpha_g$. As shown in Table~\ref{tab:fusion_ablation}, our experiments explore three aspects of the integration mechanism:

First, for architectural design, different choices for combining LSP and GSP, including sequential integration and linear fusion, show competitive but slightly inferior performance ($\sim$81.2\%) compared to our parallel processing with learnable weights. When examining weight constraints, experiments with fixed sum or single learnable weight show significant performance degradation ($\sim$80.1-80.2\%), validating our choice of independent weight optimization. Moreover, more sophisticated approaches like neural networks, gating mechanisms, and MLPs show inferior performance (80.15-80.68\%), suggesting that complex fusion strategies might introduce unnecessary optimization difficulties.

We further investigate the impact of different weight initializations between LSP and GSP branches. As shown in Fig.~\ref{fig:weight_analysis}, our analysis reveals that the best performance is achieved with balanced weight distributions ($\alpha_l = 0.5\text{--}0.6$), suggesting complementary contributions from both local and global spatial information. The model maintains robust performance (above 79.5\%) across various weight initializations, demonstrating strong stability. Notably, base classes show slight preference for higher local weights ($\alpha_l = 0.6$), while novel classes achieve optimal performance with balanced weights ($\alpha_l = 0.5$).

These comprehensive experiments yield several important insights for our framework design:
\begin{itemize}
    \item Simple learnable weights outperform complex fusion mechanisms, emphasizing flexibility over complexity
    \item Independent optimization of LSP and GSP weights is crucial for optimal performance
    \item The framework shows remarkable robustness to initialization while maintaining effective weight learning
    \item Balanced contribution from both spatial perspectives is essential for overall performance
\end{itemize}

\begin{figure}[t]
    \centering
    \includegraphics[width=0.95\linewidth]{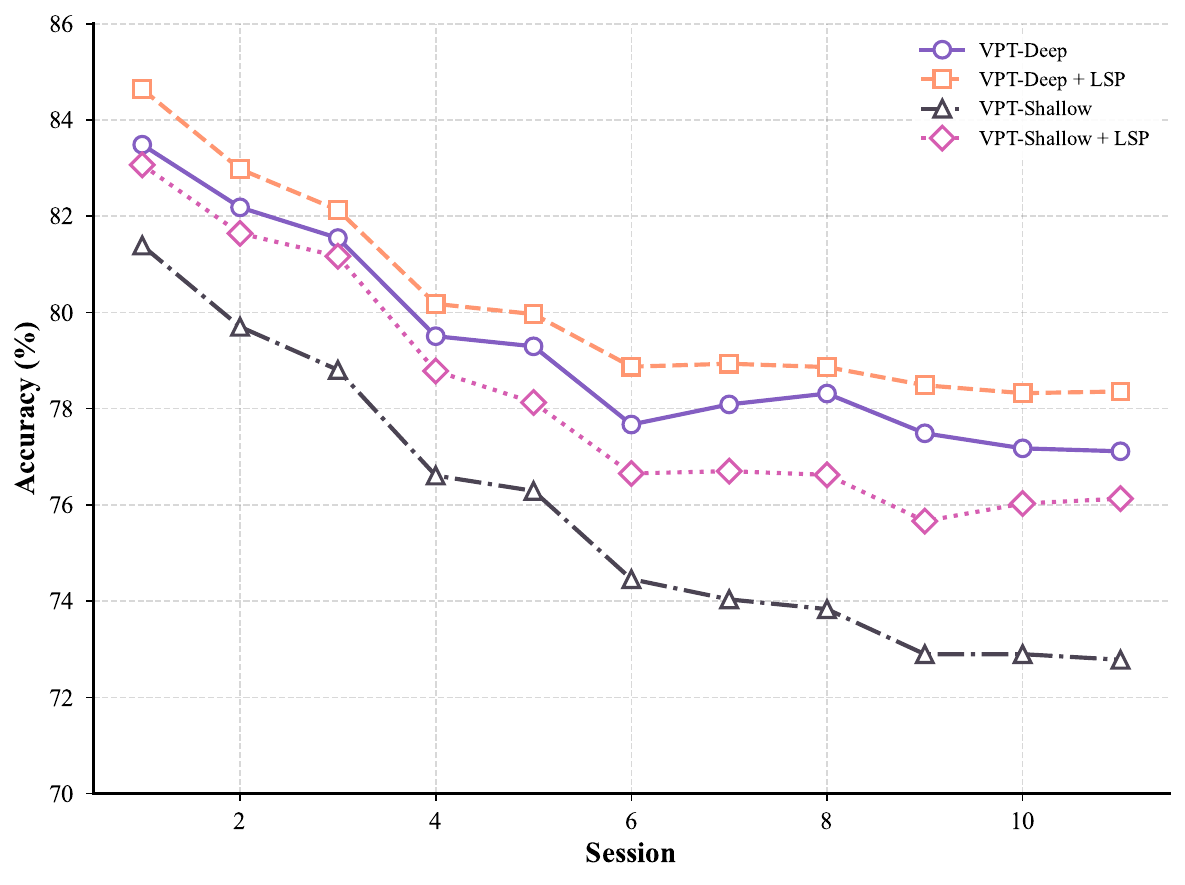}
    \caption{Performance comparison of different VPT variants across sessions. The proposed LSP module consistently improves the performance on both VPT-Deep and VPT-Shallow architectures, demonstrating its effectiveness in addressing the token-dimension saturation problem. Notably, the performance gain is more significant in the VPT-Shallow setting (+3.348\%) compared to VPT-Deep (+1.243\%), indicating LSP's particular strength in resource-constrained scenarios.}
    \label{fig:ablation_study}
\end{figure}

\subsection{Detailed Analysis of LSP's Effectiveness}

We conduct extensive experiments to validate the effectiveness of our proposed Local Spatial Prompting (LSP) module across different architectures. Table~\ref{tab:ablation_detailed} presents a detailed breakdown of the performance metrics in the final session, where we evaluate the model's capability in both within-space and cross-space classification scenarios.

Our experimental results reveal several significant findings:

\medskip
\noindent \textbf{Universal Effectiveness.} LSP demonstrates consistent performance improvements across both deep and shallow architectures. Notably, in the final session, both architectures show enhanced performance across all evaluation metrics, validating LSP's architectural versatility.

\medskip
\noindent \textbf{Enhanced Cross-space Recognition.} The B→B+N and N→B+N metrics show significant improvements with LSP. In VPT-Deep configuration, B→B+N accuracy improved by 2.23\% (81.18\% → 83.41\%) while N→B+N improved by 0.27\%. More substantial gains are observed in VPT-Shallow, with B→B+N increasing by 3.87\% and N→B+N by 2.83\%.

\medskip
\noindent \textbf{Robust Within-space Performance.} The within-space metrics (B→B and N→N) also show consistent improvements. VPT-Deep + LSP achieves 84.77\% B→B accuracy and 75.77\% N→N accuracy, while VPT-Shallow + LSP shows more significant gains, particularly in N→N performance with a 3.45\% improvement.

\medskip
\noindent \textbf{Stability Across Sessions.} As shown in Figure~\ref{fig:ablation_study}, models equipped with LSP exhibit more stable performance trajectories, particularly in later incremental stages. This stability can be attributed to the spatial dimension exploitation that effectively mitigates token-dimension saturation.

These empirical results strongly support our theoretical framework:

\begin{itemize}
    \item The comprehensive improvements in both cross-space (B→B+N, N→B+N) and within-space (B→B, N→N) metrics validate our hypothesis about token-dimension saturation and the effectiveness of spatial-dimension prompting as a solution.
    
    \item The enhanced stability in later sessions, coupled with improved N→N performance, confirms that LSP successfully maintains discriminative feature learning capability throughout the incremental learning process.
    
    \item The balanced improvements across all metrics suggest that LSP effectively manages the stability-plasticity trade-off inherent in FSCIL scenarios, particularly benefiting the challenging cross-space recognition tasks.
\end{itemize}

This comprehensive analysis demonstrates that LSP not only provides quantitative performance improvements but also addresses fundamental challenges in FSCIL through its innovative spatial prompting mechanism, especially in scenarios requiring cross-space knowledge transfer.

%-------------------------------------------------------------------------

\begin{figure}[t]
    \centering
    \includegraphics[width=0.95\linewidth]{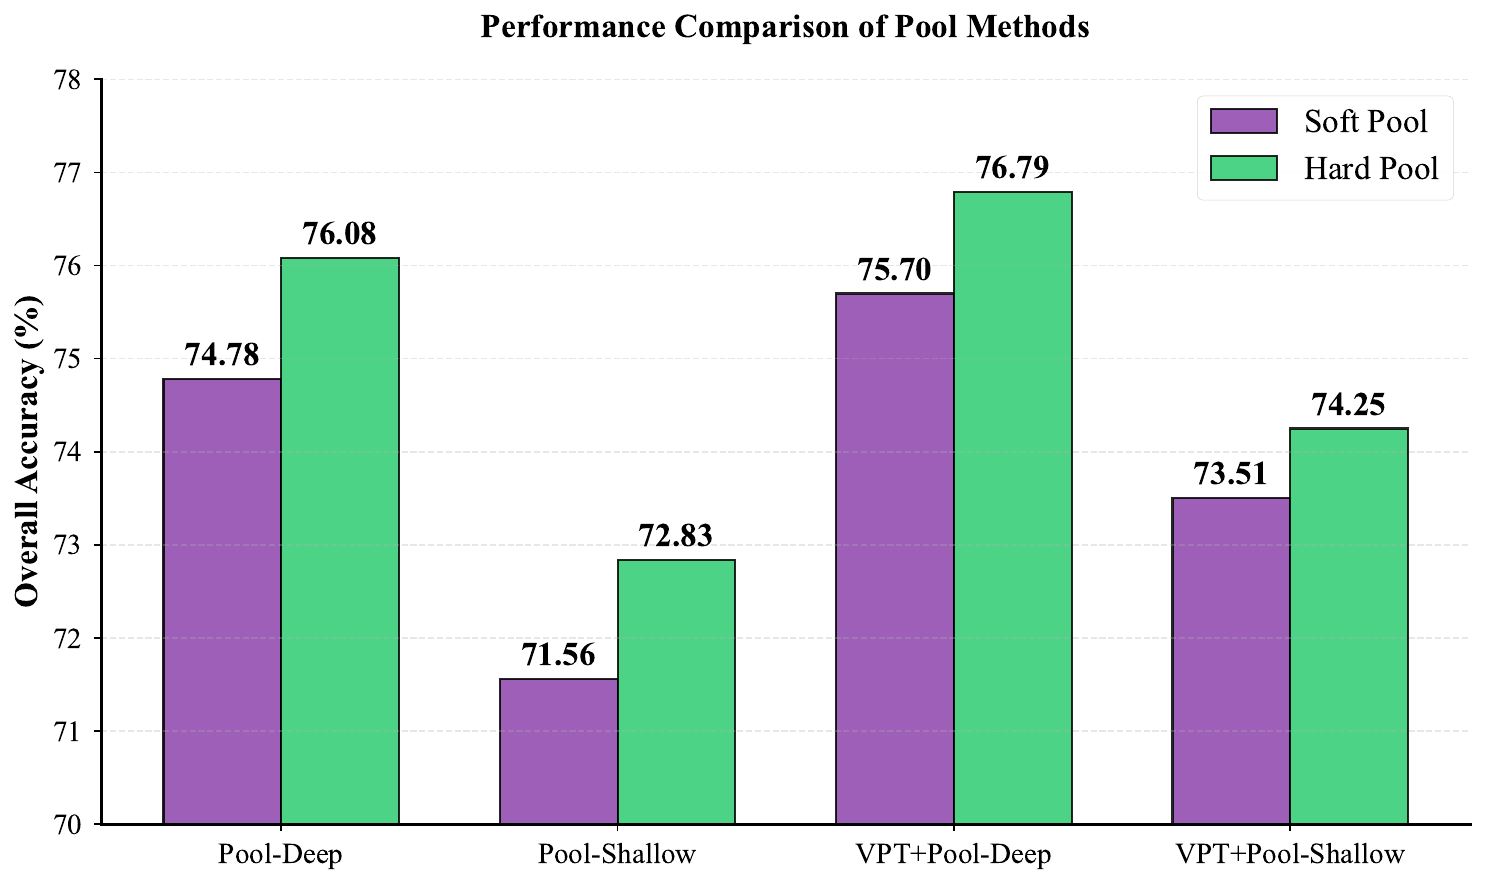}
    \caption{Performance comparison between soft and hard pooling methods. All experiments are conducted with a fixed VPT length of 5 and pool selection size of 5, which is determined based on our previous analysis showing that token-dimension conflicts emerge when the total number of prompts exceeds 10. This controlled setting allows us to: (1) maintain both VPT and pool prompts below the saturation threshold, ensuring both modules can potentially contribute positively to the model's performance, and (2) specifically investigate whether soft pooling can effectively aggregate information from all prompts in the pool without interference from saturation effects.}
    \label{fig:pool_methods_comparison}
\end{figure}

\subsection{Analysis of VPT and Pool Architecture Variants}

As illustrated in Fig.~\ref{fig:VPT_Pool_deep_shallow}, we first analyze the performance of different Visual Prompt Tuning architectures on the CUB-200 dataset. The results show that VPT-deep consistently outperforms VPT-shallow across all sessions, maintaining higher accuracy (77.2\% vs. 72.8\% at session 10) and exhibiting better stability in knowledge retention. This performance gap motivates us to extend the deep integration strategy to the pool-based mechanism, leading to the development of Pool-deep architecture for our subsequent investigation into prompt pool mechanisms for FSCIL tasks.

The superior performance of deep variants can be attributed to their hierarchical feature modulation capability, where prompts are inserted at multiple transformer layers (\(L_1\), \(L_2\), ..., \(L_N\)). This design enables the model to capture and modify features at various abstraction levels, from low-level visual patterns to high-level semantic concepts. While the original prompt pool method~\cite{wang2022learning} only utilized shallow integration at the input layer, we enhance it to Pool-deep by extending prompt insertion across multiple layers. As shown in Fig.~\ref{fig:VPT_Pool_deep_shallow}, this improvement leads to consistently better results compared to Pool-shallow (76.1\% vs. 72.9\% at session 10). The performance curves also indicate that deep architectures are more resilient to catastrophic forgetting, maintaining more stable accuracy across incremental sessions.
%-------------------------------------------------------------------------

\begin{table}[t]
\centering
\small
\caption{Detailed performance comparison of LSP across different architectures in the final session. 
B→B+N denotes the accuracy of base classes' logits mapped to both base and novel classes space; 
N→B+N represents novel classes' logits mapped to the complete class space; 
B→B indicates base classes' accuracy within base class space; 
N→N shows novel classes' accuracy within novel class space.}
\label{tab:ablation_detailed}
\setlength{\tabcolsep}{3pt}
\begin{tabular}{l|cccc}
\toprule
\textbf{Model} & \textbf{B→B+N} & \textbf{N→B+N} & \textbf{B→B} & \textbf{N→N} \\
\midrule
VPT-Deep & 81.18 & 73.14 & 84.71 & 73.92 \\
VPT-Deep + LSP & \textbf{83.41} & \textbf{73.41} & \textbf{84.77} & \textbf{75.77} \\
\midrule
VPT-Shallow & 78.25 & 67.44 & 81.60 & 69.01 \\
VPT-Shallow + LSP & \textbf{82.12} & \textbf{70.27} & \textbf{83.28} & \textbf{72.46} \\
\bottomrule
\end{tabular}
\end{table}

\begin{figure*}[!ht]
    \centering
    \begin{minipage}{0.48\textwidth}
        \centering
        \begin{tikzpicture}
            \begin{axis}[
                title={\large VPT Performance},
                xlabel={\large Session},
                ylabel={\large Accuracy (\%)},
                grid=both,
                grid style={line width=.1pt, draw=gray!20},
                major grid style={line width=.2pt,draw=gray!50},
                xtick={0,1,...,10},
                ytick={70,72.5,75,77.5,80,82.5,85},
                ymin=70, ymax=85,
                width=8.5cm,
                height=6.5cm,
                cycle list={blue, red},
                mark options={solid, scale=1.2},
                legend pos=south west,
                legend style={font=\small, fill=white, fill opacity=0.8, draw=none},
                every axis plot/.append style={line width=1.2pt},
                tick label style={font=\small},
                title style={font=\normalsize\bfseries},
                label style={font=\normalsize}
            ]
            % VPT-deep
            \addplot[mark=*, thick, color=blue!80!black] coordinates {(0,83.485) (1,82.183) (2,81.545) (3,79.506) (4,79.295) (5,77.67) (6,78.088) (7,78.314) (8,77.488) (9,77.175) (10,77.114)};
            \addlegendentry{\textbf{VPT-deep}}

            % VPT-shallow
            \addplot[mark=*, thick, color=red!80!black] coordinates {(0,81.39) (1,79.701) (2,78.805) (3,76.609) (4,76.291) (5,74.457) (6,74.036) (7,73.834) (8,72.897) (9,72.898) (10,72.782)};
            \addlegendentry{\textbf{VPT-shallow}}
            \end{axis}
        \end{tikzpicture}
    \end{minipage}
    \hfill
    \begin{minipage}{0.48\textwidth}
        \centering
        \begin{tikzpicture}
            \begin{axis}[
                title={\large Pool Performance},
                xlabel={\large Session},
                ylabel={\large Accuracy (\%)},
                grid=both,
                grid style={line width=.1pt, draw=gray!20},
                major grid style={line width=.2pt,draw=gray!50},
                xtick={0,1,...,10},
                ytick={70,72.5,75,77.5,80,82.5,85},
                ymin=70, ymax=85,
                width=8.5cm,
                height=6.5cm,
                cycle list={green, orange},
                mark options={solid, scale=1.2},
                legend pos=south west,
                legend style={font=\small, fill=white, fill opacity=0.8, draw=none},
                every axis plot/.append style={line width=1.2pt},
                tick label style={font=\small},
                title style={font=\normalsize\bfseries},
                label style={font=\normalsize}
            ]
            % pool-deep
            \addplot[mark=*, thick, color=green!60!black] coordinates {(0,81.983) (1,80.751) (2,79.563) (3,77.951) (4,77.731) (5,76.745) (6,76.983) (7,76.766) (8,75.951) (9,75.755) (10,76.079)};
            \addlegendentry{\textbf{Pool-deep}}

            % pool-shallow
            \addplot[mark=*, thick, color=orange!90!black] coordinates {(0,81.18) (1,79.478) (2,78.601) (3,76.046) (4,75.645) (5,73.948) (6,73.754) (7,73.081) (8,72.589) (9,72.734) (10,72.834)};
            \addlegendentry{\textbf{Pool-shallow}}
            \end{axis}
        \end{tikzpicture}
    \end{minipage}
    \caption{Performance comparison of VPT and Pool methods on the CUB-200 dataset. Both approaches demonstrate superior performance with deep configuration, showing consistent advantages in maintaining accuracy across incremental sessions. The deep variants (VPT-deep and Pool-deep) consistently outperform their shallow counterparts, with VPT-deep achieving the best overall performance and exhibiting more stable accuracy retention.}
    \label{fig:VPT_Pool_deep_shallow}
\end{figure*}

\subsection{Analysis of Soft Pool vs. Hard Pool Methods}

Motivated by our visualization analysis that revealed token-dimension saturation issues, we conducted experiments comparing soft and hard pooling strategies. The soft pooling approach attempts to address the saturation problem by computing similarity-based weighted combinations of prompts, potentially allowing the model to utilize information from multiple prompts while avoiding direct token-dimension conflicts.

As shown in Figure~\ref{fig:pool_methods_comparison}, our experimental results with carefully controlled prompt numbers (VPT length = 5, selected pool size = 5) reveal several key findings:

\textbf{Consistent Performance Gap:} Even in this controlled setting where token-dimension saturation is avoided, hard pooling consistently outperforms soft pooling across all configurations. The performance gap (1.30\% improvement in Pool-Deep, 1.09\% in VPT-Pool-Deep) suggests that the limitations of soft pooling are not merely due to token saturation but rather inherent to the weighted combination approach itself.

\textbf{VPT Integration Benefits:} The integration of VPT (length = 5) with pool-based methods shows improved performance in both variants, with VPT-Pool-Deep achieving the best results (75.70\% for soft, 76.79\% for hard). This indicates that the initialized VPT prompts provide complementary features to the selected pool prompts when their total number is kept below the saturation threshold.

\textbf{Architecture Impact:} Deep architectures demonstrate superior performance across both pooling strategies, suggesting better capability in utilizing the limited number of prompts effectively.

These findings indicate that while soft pooling was designed to potentially leverage information from all prompts through weighted combinations, it fails to outperform the direct selection mechanism of hard pooling even in scenarios carefully designed to avoid token-dimension saturation. This suggests that the challenge lies not in the quantity of information that can be stored in the token dimension, but rather in how effectively this information can be utilized. The superior performance of hard pooling, even with the same number of prompts, supports our motivation to explore alternative dimensions for prompt learning rather than attempting to optimize information aggregation within the token dimension.
%-------------------------------------------------------------------------

\begin{figure*}[p]
    \centering
    % Row 1
    \begin{minipage}{2\columnwidth}
        \centering
        \includegraphics[width=0.16\textwidth]{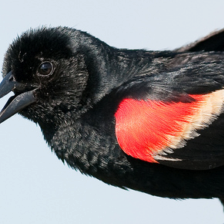}
        \includegraphics[width=0.16\textwidth]{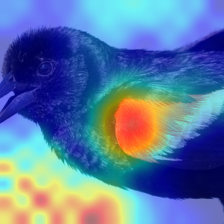}
        \includegraphics[width=0.16\textwidth]{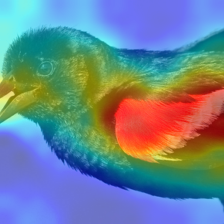}
        \includegraphics[width=0.16\textwidth]{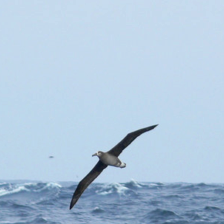}
        \includegraphics[width=0.16\textwidth]{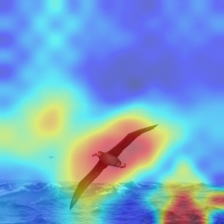}
        \includegraphics[width=0.16\textwidth]{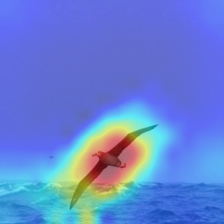}
    \end{minipage}
    
    \vspace{0.8mm}
    % Row 2
    \begin{minipage}{2\columnwidth}
        \centering
        \includegraphics[width=0.16\textwidth]{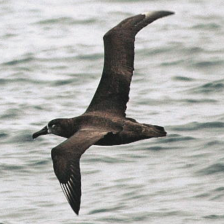}
        \includegraphics[width=0.16\textwidth]{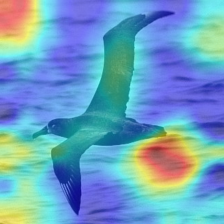}
        \includegraphics[width=0.16\textwidth]{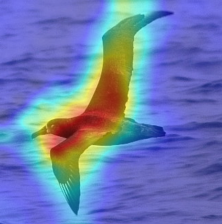}
        \includegraphics[width=0.16\textwidth]{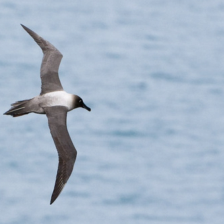}
        \includegraphics[width=0.16\textwidth]{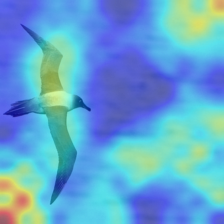}
        \includegraphics[width=0.16\textwidth]{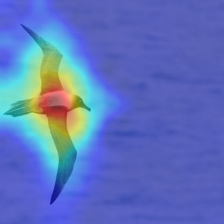}
    \end{minipage}

    \vspace{0.8mm}
    % Row 3
    \begin{minipage}{2\columnwidth}
        \centering
        \includegraphics[width=0.16\textwidth]{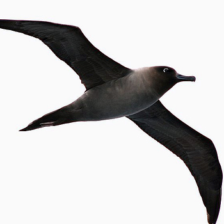}
        \includegraphics[width=0.16\textwidth]{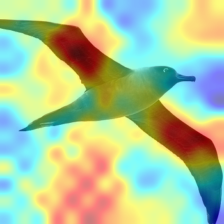}
        \includegraphics[width=0.16\textwidth]{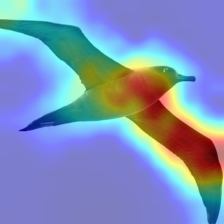}
        \includegraphics[width=0.16\textwidth]{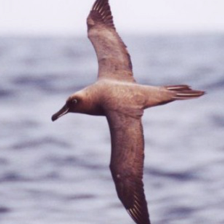}
        \includegraphics[width=0.16\textwidth]{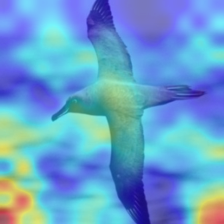}
        \includegraphics[width=0.16\textwidth]{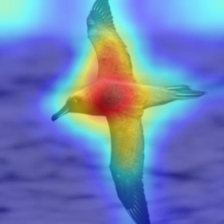}
    \end{minipage}

    \vspace{0.8mm}
    % Row 4
    \begin{minipage}{2\columnwidth}
        \centering
        \includegraphics[width=0.16\textwidth]{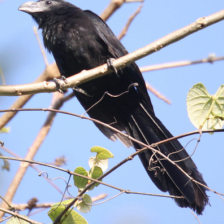}
        \includegraphics[width=0.16\textwidth]{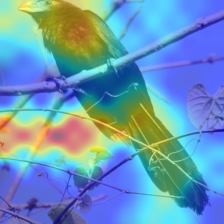}
        \includegraphics[width=0.16\textwidth]{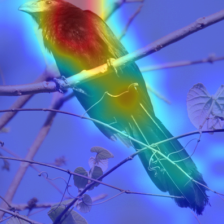}
        \includegraphics[width=0.16\textwidth]{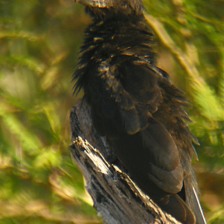}
        \includegraphics[width=0.16\textwidth]{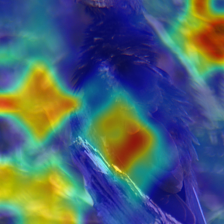}
        \includegraphics[width=0.16\textwidth]{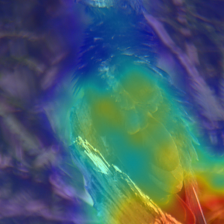}
    \end{minipage}

    \vspace{0.8mm}
    % Row 5
    \begin{minipage}{2\columnwidth}
        \centering
        \includegraphics[width=0.16\textwidth]{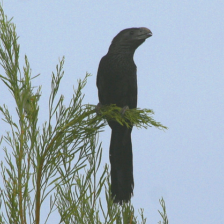}
        \includegraphics[width=0.16\textwidth]{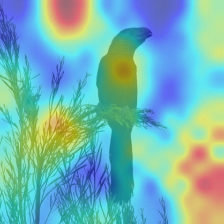}
        \includegraphics[width=0.16\textwidth]{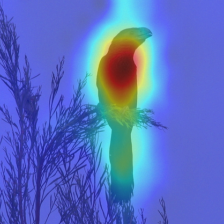}
        \includegraphics[width=0.16\textwidth]{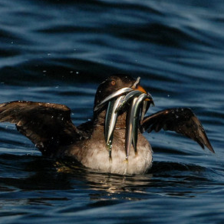}
        \includegraphics[width=0.16\textwidth]{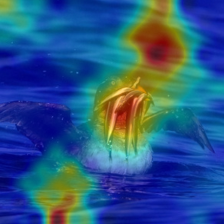}
        \includegraphics[width=0.16\textwidth]{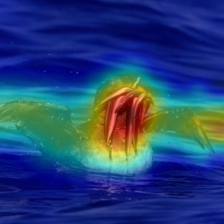}
    \end{minipage}

    \vspace{0.8mm}
    % Row 4
    \begin{minipage}{2\columnwidth}
        \centering
        \includegraphics[width=0.16\textwidth]{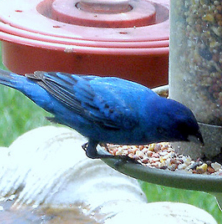}
        \includegraphics[width=0.16\textwidth]{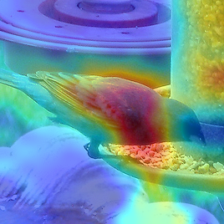}
        \includegraphics[width=0.16\textwidth]{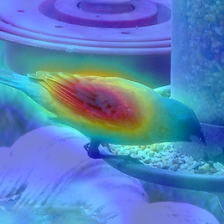}
        \includegraphics[width=0.16\textwidth]{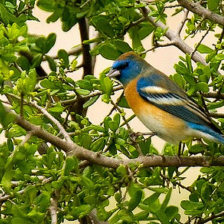}
        \includegraphics[width=0.16\textwidth]{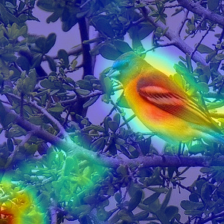}
        \includegraphics[width=0.16\textwidth]{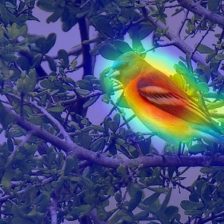}
    \end{minipage}

    \vspace{0.8mm}
    % Row 4
    \begin{minipage}{2\columnwidth}
        \centering
        \includegraphics[width=0.16\textwidth]{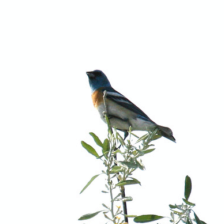}
        \includegraphics[width=0.16\textwidth]{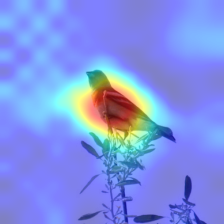}
        \includegraphics[width=0.16\textwidth]{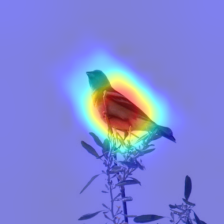}
        \includegraphics[width=0.16\textwidth]{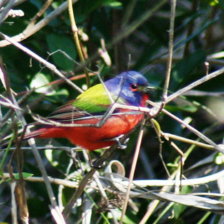}
        \includegraphics[width=0.16\textwidth]{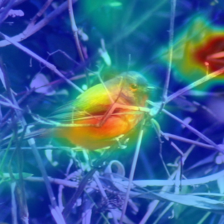}
        \includegraphics[width=0.16\textwidth]{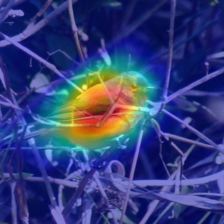}
    \end{minipage}
    
    \vspace{2mm}
    {\small
    \makebox[0.16\textwidth]{orig}
    \makebox[0.16\textwidth]{cls}
    \makebox[0.16\textwidth]{pmt}
    \makebox[0.16\textwidth]{orig}
    \makebox[0.16\textwidth]{cls}
    \makebox[0.16\textwidth]{pmt}
    }
    
    \caption{Extended visualization of attention patterns (Part 1). For each group of three images: orig shows the original input image, cls displays the class token attention heat map before applying our method, and pmt shows the prompt attention heat map after applying our Local Spatial Prompting mechanism.}
    \label{fig:attention_maps_extended_1}
\end{figure*}

\begin{figure*}[p]
    \centering
    % Row 1
    \begin{minipage}{2\columnwidth}
        \centering
        \includegraphics[width=0.16\textwidth]{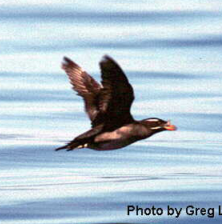}
        \includegraphics[width=0.16\textwidth]{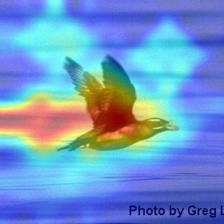}
        \includegraphics[width=0.16\textwidth]{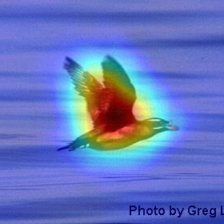}
        \includegraphics[width=0.16\textwidth]{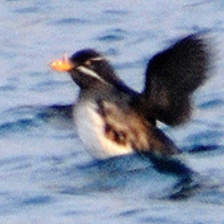}
        \includegraphics[width=0.16\textwidth]{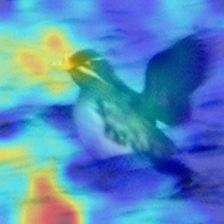}
        \includegraphics[width=0.16\textwidth]{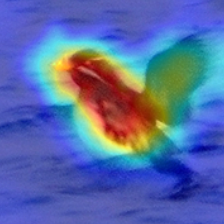}
    \end{minipage}

    \vspace{0.8mm}
    % Row 2
    \begin{minipage}{2\columnwidth}
        \centering
        \includegraphics[width=0.16\textwidth]{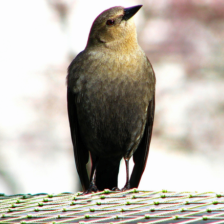}
        \includegraphics[width=0.16\textwidth]{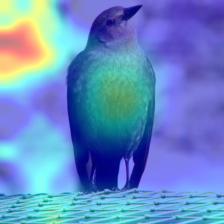}
        \includegraphics[width=0.16\textwidth]{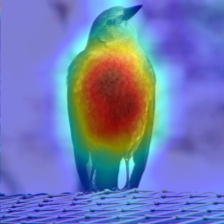}
        \includegraphics[width=0.16\textwidth]{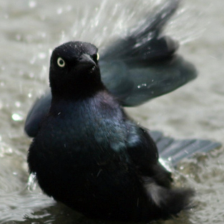}
        \includegraphics[width=0.16\textwidth]{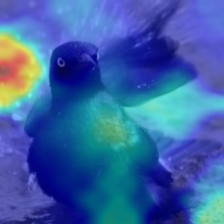}
        \includegraphics[width=0.16\textwidth]{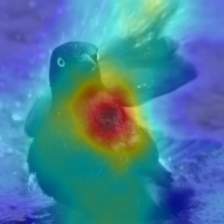}
    \end{minipage}

    \vspace{0.8mm}
    % Row 3
    \begin{minipage}{2\columnwidth}
        \centering
        \includegraphics[width=0.16\textwidth]{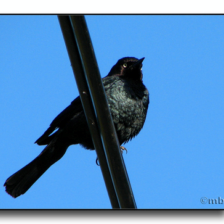}
        \includegraphics[width=0.16\textwidth]{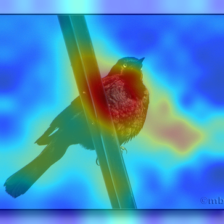}
        \includegraphics[width=0.16\textwidth]{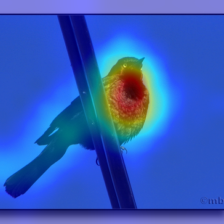}
        \includegraphics[width=0.16\textwidth]{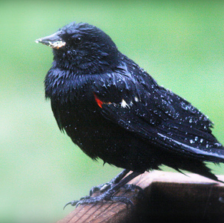}
        \includegraphics[width=0.16\textwidth]{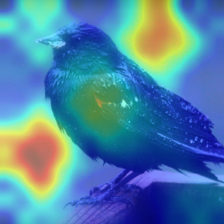}
        \includegraphics[width=0.16\textwidth]{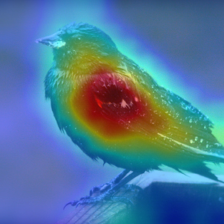}
    \end{minipage}

    % Row 3
    \begin{minipage}{2\columnwidth}
        \centering
        \includegraphics[width=0.16\textwidth]{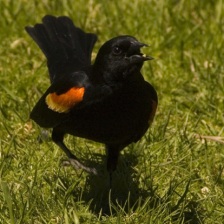}
        \includegraphics[width=0.16\textwidth]{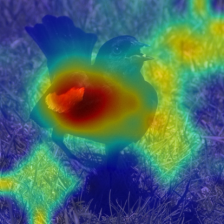}
        \includegraphics[width=0.16\textwidth]{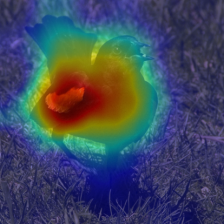}
        \includegraphics[width=0.16\textwidth]{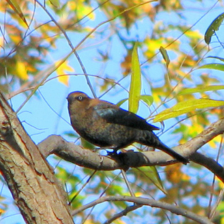}
        \includegraphics[width=0.16\textwidth]{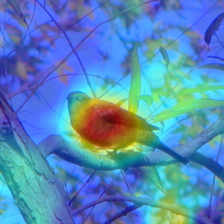}
        \includegraphics[width=0.16\textwidth]{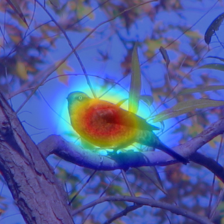}
    \end{minipage}

    \vspace{0.8mm}
    % Row 4
    \begin{minipage}{2\columnwidth}
        \centering
        \includegraphics[width=0.16\textwidth]{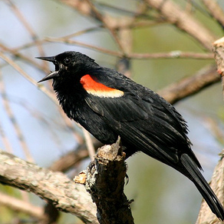}
        \includegraphics[width=0.16\textwidth]{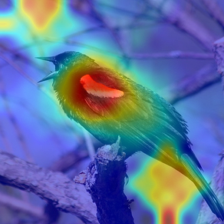}
        \includegraphics[width=0.16\textwidth]{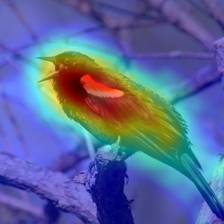}
        \includegraphics[width=0.16\textwidth]{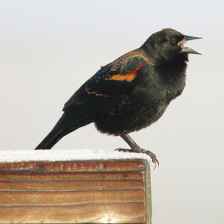}
        \includegraphics[width=0.16\textwidth]{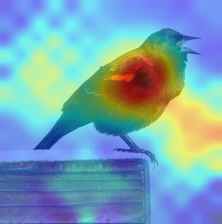}
        \includegraphics[width=0.16\textwidth]{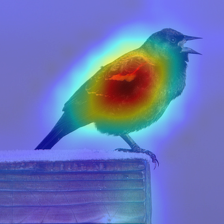}
    \end{minipage}

    \vspace{0.8mm}
    % Row 4
    \begin{minipage}{2\columnwidth}
        \centering
        \includegraphics[width=0.16\textwidth]{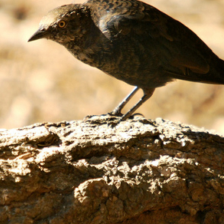}
        \includegraphics[width=0.16\textwidth]{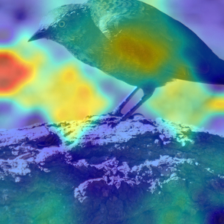}
        \includegraphics[width=0.16\textwidth]{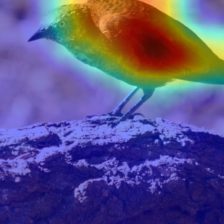}
        \includegraphics[width=0.16\textwidth]{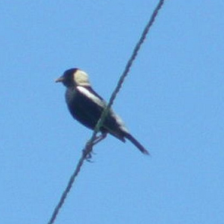}
        \includegraphics[width=0.16\textwidth]{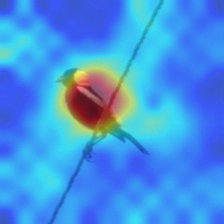}
        \includegraphics[width=0.16\textwidth]{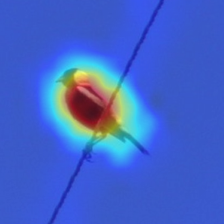}
    \end{minipage}

    \vspace{0.8mm}
    % Row 4
    \begin{minipage}{2\columnwidth}
        \centering
        \includegraphics[width=0.16\textwidth]{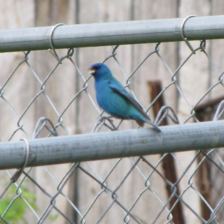}
        \includegraphics[width=0.16\textwidth]{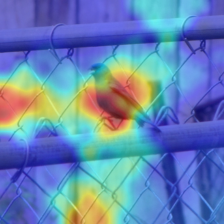}
        \includegraphics[width=0.16\textwidth]{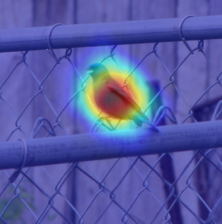}
        \includegraphics[width=0.16\textwidth]{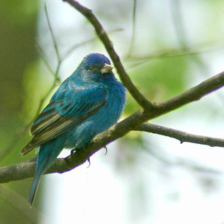}
        \includegraphics[width=0.16\textwidth]{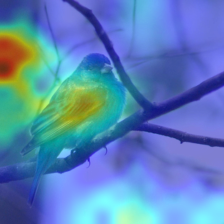}
        \includegraphics[width=0.16\textwidth]{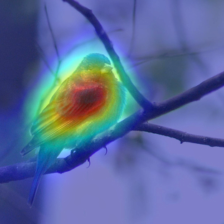}
    \end{minipage}
    
    \vspace{2mm}
    {\small
    \makebox[0.16\textwidth]{orig}
    \makebox[0.16\textwidth]{cls}
    \makebox[0.16\textwidth]{pmt}
    \makebox[0.16\textwidth]{orig}
    \makebox[0.16\textwidth]{cls}
    \makebox[0.16\textwidth]{pmt}
    }
    
    \caption{Extended visualization of attention patterns (Part 2). The visualization demonstrates consistent improvement in attention focus across diverse samples, with the model learning to attend to discriminative features rather than background elements.}
    \label{fig:attention_maps_extended_2}
\end{figure*}
%-------------------------------------------------------------------------
%-------------------------------------------------------------------------
\section{Extended Attention Pattern Analysis}

We provide an extended visualization of attention patterns in Figures~\ref{fig:attention_maps_extended_1} and~\ref{fig:attention_maps_extended_2} to further demonstrate the effectiveness of our Local Spatial Prompting mechanism across a diverse set of samples. These additional examples consistently show how our approach reshapes the attention distribution, shifting focus from background elements to semantically meaningful regions of the target objects.

In these extended examples, we observe several key patterns:

\textbf{Consistent Focus Improvement:} Across all samples, the prompt attention maps (pmt) show more precise focus on the target objects compared to the baseline class token attention (cls).

\textbf{Background Suppression:} Our method effectively reduces attention to irrelevant background elements, which is particularly evident in samples with complex or cluttered backgrounds.

\textbf{Feature Highlighting:} The prompt attention maps consistently highlight discriminative features of the objects, suggesting that our Local Spatial Prompting mechanism helps the model learn more robust and relevant feature representations.

These additional visualizations further support our main findings and demonstrate the generalizability of our approach across different scenarios and object types.

%-------------------------------------------------------------------------

\section{Limitations}
While our proposed Local-Global Spatial Prompt Framework offers significant advancements in addressing the token dimension saturation problem in Few-Shot Class Incremental Learning (FSCIL), several limitations warrant discussion:

\textbf{Memory Overhead from Buffering:} The introduction of a buffer for maintaining spatial prompts may lead to additional memory overhead. This raises questions about the efficiency of resource utilization, particularly in environments with constrained computational resources.

\textbf{Dependence on Adequate Pre-training:} Our framework assumes that adequate pre-training is available to provide meaningful representations. However, in certain applications, such as those with limited labeled data or in rapidly changing environments, this assumption may not hold, potentially impacting the model's performance.

\textbf{Applicability to Transformer Architectures:} The prompt-based strategy is primarily designed for transformer backbones, which may limit its applicability to other architectures. This raises concerns about the generalizability of our approach across different model types, particularly in scenarios where non-transformer architectures are preferred.

\textbf{Frozen Transformer Backbone:} The transformer backbone in our framework is frozen and adapted to downstream tasks solely through prompt parameters. This design choice restricts the enrichment and updating of pre-trained knowledge, potentially limiting the model's ability to adapt to new information or tasks effectively.

By acknowledging these limitations, we aim to provide a balanced perspective on the strengths and weaknesses of our proposed framework, paving the way for future research to address these challenges and enhance the applicability of our approach in diverse settings.
